# Supplementary material for: High-Throughput Screening of 2D Photocatalyst Heterostructures with Suppressed Electron-Hole Recombination for Solar Water Splitting
Source: arXiv:2508.17483 ancillary file (2025-08-24)
Supplement: Supplementary file 1 [file SI.pdf]

# Supporting Information
# High-Throughput Screening of 2D Photocatalyst Heterostructures with Suppressed Electron–Hole Recombination for Solar Water Splitting

Shivanand Yadav,[1] Jainandan Kumar Modi,[2] Raihan Ahammed,[3] B. S. Bhadoria,[1] Yogesh S. Chauhan,[2] Amit Agarwal,[3,*] and Somnath Bhowmick[4,†]

[1]*Department of Physics, Bundelkhand University, Jhansi 284128, India*

[2]*Department of Electrical Engineering, Indian Institute of Technology, Kanpur, Kanpur 208016, India*

[3]*Department of Physics, Indian Institute of Technology, Kanpur, Kanpur 208016, India*

[4]*Department of Materials Science & Engineering, Indian Institute of Technology, Kanpur, Kanpur 208016, India*

(Dated: July 24, 2025)

* amitag@iitk.ac.in

† bsomnath@iitk.ac.in

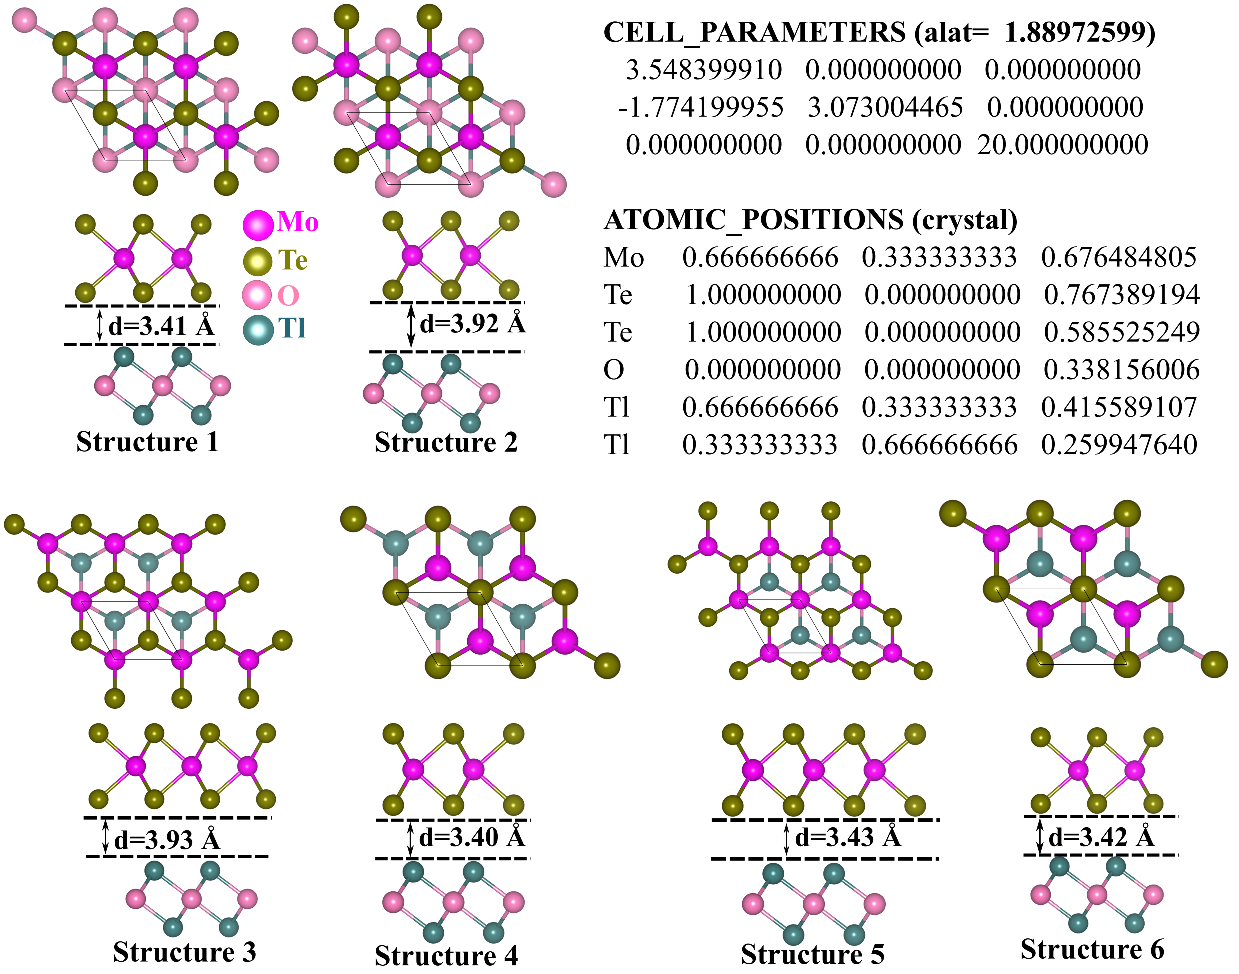


FIG. S1. Top and side view of six different stacking patterns of $MoTe_2/Tl_2O$, obtained by rotating monolayers at angles of 0° (structure 1), 60° (structure 2), 120° (structure 3), 180° (structure 4), 240° (structure 5), and 300° (structure 6) with respect to each other. Among all, structure 4 (cell parameters and atomic positions given) is the most stable configuration, having the lowest ground state energy.

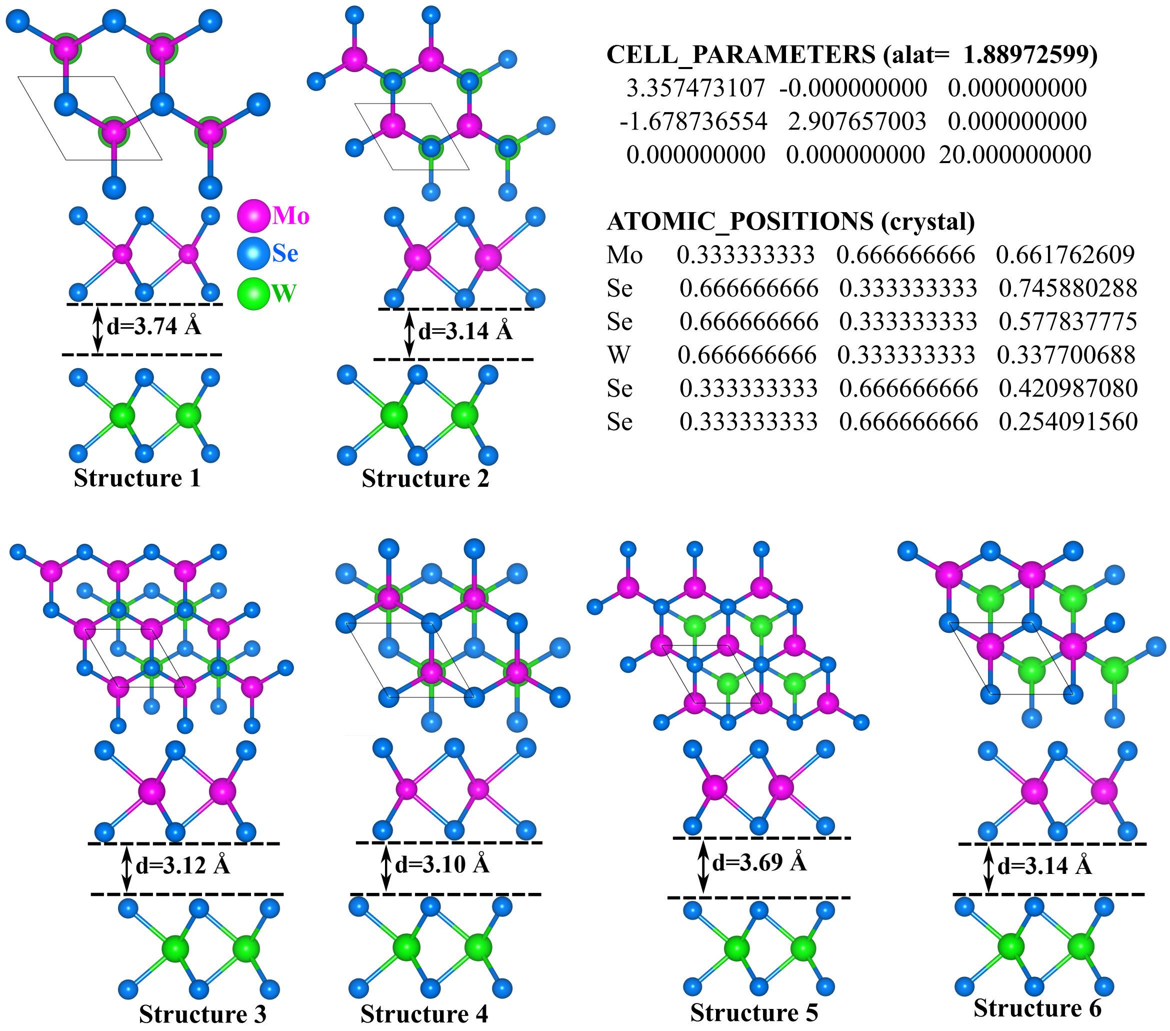


FIG. S2. Top and side view of six different stacking patterns of $MoSe_2/WSe_2$, obtained by rotating monolayers at angles of 0° (structure 1), 60° (structure 2), 120° (structure 3), 180° (structure 4), 240° (structure 5), and 300° (structure 6) with respect to each other. Among all, structure 2 (cell parameters and atomic positions given) is the most stable configuration, having the lowest ground state energy.

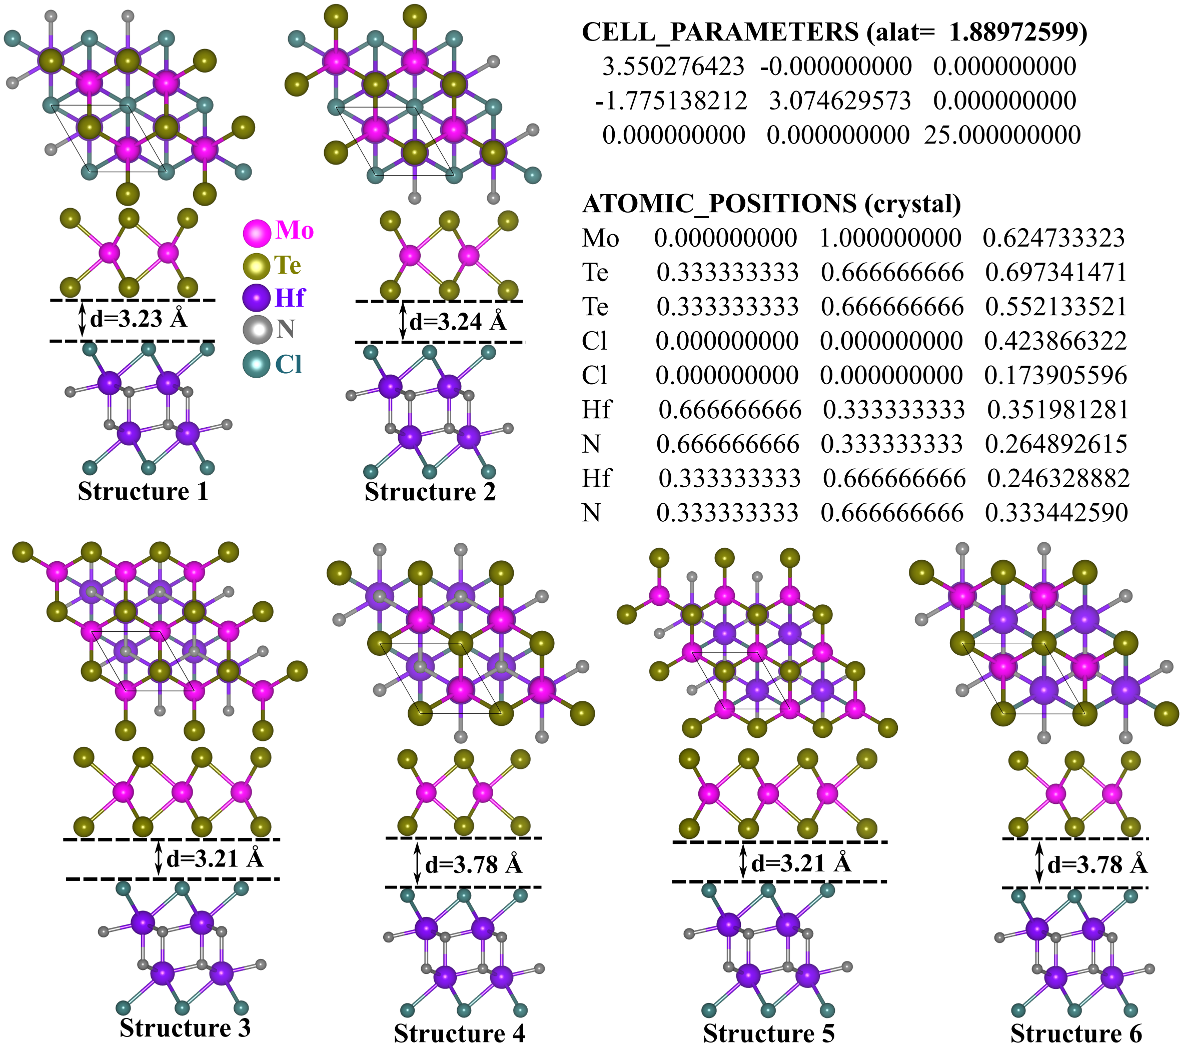


FIG. S3. Top and side view of six different stacking patterns of $MoTe_2$/HfNCl, obtained by rotating monolayers at angles of 0° (structure 1), 60° (structure 2), 120° (structure 3), 180° (structure 4), 240° (structure 5), and 300° (structure 6) with respect to each other. Among all, structure 5 (cell parameters and atomic positions given) is the most stable configuration, having the lowest ground state energy.

## S1. CRYSTAL GEOMETRY OF THE HETEROSTRUCTURES

$MoTe_2/Tl_2O$ heterostructure: $MoTe_2$ and $Tl_2O$ monolayers have closely matched lattice parameters of 3.56 Å and 3.57 Å, respectively, resulting in a very small lattice mismatch of about 0.28%. Among different stacking sequences, structure 4 has the lowest energy, with bond lengths of 2.74 Å (Mo–Te) and 2.57 Å (Tl–O), a binding energy of –36.87 meV/Å$^2$, and an optimal interlayer distance of 3.40 Å (Fig. S1).

$MoSe_2/WSe_2$ heterostructure: $MoSe_2$ and $WSe_2$ monolayers have closely matched lattice parameters of 3.31 Å and 3.31 Å, respectively. Among different stacking sequences, structure 2 has the lowest total energy, with bond lengths of 2.56 Å (Mo–Se) and 2.55 Å (W–Se), a binding energy of -28.32 meV/Å$^2$, and an optimal interlayer distance of 3.14 Å (Fig. S2).

$MoTe_2$/HfNCl heterostructure: $MoTe_2$ and HfNCl monolayers have closely matched lattice parameters of 3.56 Å and 3.57 Å, respectively, resulting in a very small lattice mismatch of about 0.28%. Among different stacking sequences, structure 5 has the lowest total energy, with bond lengths of 2.74 Å (Mo–Te), 2.73 Å (Hf–Cl), and 2.10 Å (Hf–N), a binding energy of -24.55 meV/Å$^2$, and an optimal interlayer distance of 3.21 Å (Fig. S3).

TABLE SI. Optimized lattice parameters a (in Å), Interlayer distance d (in Å), Band gap $E_g$ (in eV) with HSE06 (in bracket PBE) , and Binding energy(meV/Å$^2$) of heterostructure.

| Materials | $a(=b)$ (Å) | $d$ (Å) | $E_g(eV)$ | Binding Energy($meV/\AA^2$) | Materials | $a(=b)$ (Å) | $d$ (Å) | $E_g(eV)$ | Binding Energy($meV/\AA^2$) |
|---|---|---|---|---|---|---|---|---|---|
| $MoTe_2$-$Tl_2O$ | 3.55 | 3.40 | 1.49 (0.96) | -36.87 | $ZnI_2$-CuI | 4.06 | 3.34 | 1.59 (0.70) | -18.73 |
| $MoSe_2$-$WSe_2$ | 3.36 | 3.14 | 1.85 (1.04) | -28.32 | SiH-$CdBr_2$ | 3.89 | 2.14 | 2.84 (1.59) | -8.74 |
| $MoTe_2$-HfNCl | 3.55 | 3.21 | 1.43 (0.62) | -24.55 | $CdBr_2$-CuI | 4.05 | 3.18 | 1.79 (0.76) | -4.86 |
| $PtS_2$-$MoTe_2$ | 3.57 | 2.86 | 1.43 (0.81) | -33.94 | YOCl-SiH | 3.79 | 2.22 | 2.32 (1.30) | -6.44 |
| $MoS_2$-$WS_2$ | 3.19 | 3.03 | 2.04 (1.09) | -24.39 | GaSe-$CdCl_2$ | 3.76 | 3.12 | 2.91 (1.81) | -11.96 |
| HfNCl-$Tl_2O$ | 3.56 | 3.21 | 1.63 (0.52) | -31.61 | GaS-GaSe | 3.66 | 3.14 | 2.59 (1.73) | -7.85 |
| $WS_2$-P | 3.22 | 3.09 | 2.12 (1.14) | -16.27 | $CdCl_2$-SiH | 3.84 | 2.01 | 2.41 (1.19) | -7.53 |
| $PtO_2$-$WS_2$ | 3.18 | 2.38 | 1.69 (0.44) | -48.93 | $CdOH_2$-GaS | 4.05 | 2.00 | 2.21 ( 1.03) | -14.23 |
| P-$MoSe_2$ | 3.31 | 3.13 | 2.26 (0.99) | -17.14 | $FeCl_2$-$CdOH_2$ | 3.44 | 1.96 | 2.31 ( 0.41) | -9.31 |
| P-$WSe_2$ | 3.34 | 3.03 | 2.15 (0.54) | -20.74 | $ZnBr_2$-SiH | 3.8 | 2.2 | 2.52 (1.38) | -7.53 |
| $Tl_2O$-HfNI | 3.66 | 3.42 | 1.85 (0.77) | -34.35 | $ZnI_2$-$CdI_2$ | 4.1 | 3.39 | 2.47 (1.87) | -13.12 |
| CuI-$CdI_2$ | 4.15 | 3.31 | 1.92 (1.04) | -17.06 | $MgOH_2$-P | 3.21 | 2.29 | 2.41 (0.85) | -5.72 |
| Sb-$CdI_2$ | 4.13 | 3.22 | 1.66 (0.92) | -17.76 | HfNBr-HfNI | 3.63 | 3.28 | 1.62 (0.67) | -26.31 |
| $CdOH_2$-$PtSe_2$ | 3.65 | 1.80 | 2.20 (0.92) | -18.30 | InSe-CuI | 4.02 | 3.14 | 1.56 (0.56) | -18.24 |
| $PtSe_2$-SiH | 3.77 | 1.99 | 1.82 (0.72) | -12.23 | InSe-$GeI_2$ | 4.03 | 3.16 | 2.00 (1.23) | -11.81 |
| $PtO_2$-$MoS_2$ | 3.19 | 2.45 | 1.82 (0.58) | -36.30 | ZrNCl-GaS | 3.58 | 3.21 | 2.3 (1.41) | -13.65 |
| $PtS_2$-$SnS_2$ | 3.63 | 2.68 | 2.22 (0.83) | -18.70 | GaS-ZrNBr | 3.61 | 3.21 | 2.35 (1.44) | -12.27 |
| $PtS_2$-ZrNBr | 3.61 | 2.98 | 2.22 (1.37) | -21.16 | $CdOH_2$-HfNBr | 3.58 | 2.00 | 1.95 (0.63) | -20.90 |
| BiTeCl-$CaI_2$ | 4.28 | 3.03 | 2.44 (1.62) | -8.52 | $CdOH_2$-HfNCl | 3.55 | 1.86 | 1.83 (0.49) | -19.53 |
| BiTeCl-$CdI_2$ | 4.19 | 3.02 | 2.34 (1.57) | -13.81 | $CdOH_2$-$ZnCl_2$ | 3.53 | 1.98 | 3.1 (1.29) | -12.1 |
| $MgOH_2$-$MoS_2$ | 3.17 | 2.18 | 2.59 (0.69) | -13.69 | $MgI_2$-CuI | 4.12 | 3.37 | 3.39 (1.99) | -17.85 |
| $PtS_2$-ZrNCl | 3.58 | 2.93 | 2.36 (1.35) | -18.10 | ZrNCl-ZrNBr | 3.61 | 3.17 | 2.51 (1.42) | -11.82 |
| $PtS_2$-HfNI | 3.64 | 2.96 | 1.57 (0.65) | -28.73 | $CaOH_2$-ZrNBr | 3.62 | 1.98 | 2.07 (0.51) | -13.22 |
| $ZnI_2$-$GeI_2$ | 4.08 | 3.39 | 2.07 (1.40) | -13.82 | HfNBr-ZrNBr | 3.6 | 3.2 | 2.59 (1.51) | -19.78 |
| $MgOH_2$-$WS_2$ | 3.16 | 2.02 | 2.76 (1.11) | -18.54 | $CaOH_2$-GaS | 3.56 | 2.00 | 3.02 (1.49) | -11.49 |
| $GeI_2$-$CdI_2$ | 4.18 | 3.34 | 2.54 (1.88) | -15.39 | $CaOH_2$-ZrNCl | 3.59 | 1.97 | 1.81 (0.31) | -11.00 |
| CuI-$GeI_2$ | 4.14 | 3.31 | 2.33 (1.39) | -17.33 | HfNBr-ZrNCl | 3.59 | 3.1 | 2.43 (1.34) | -17.32 |
| SiH-InSe | 3.90 | 1.96 | 2.57 (1.48) | -10.72 | HfNCl-ZrNCl | 3.57 | 3.01 | 2.92 (1.78) | -15.93 |
| HfNBr-$HfS_2$ | 3.60 | 2.98 | 2.63 (1.11) | -25.86 | HfNCl-HfNBr | 3.57 | 3.01 | 3.12 (1.95) | -25.63 |
| $HfS_2$-GaSe | 3.68 | 2.99 | 1.58 (0.80) | -17.96 | HfNCl-$CaOH_2$ | 3.56 | 1.99 | 2.54 (0.87) | -15.23 |
| InSe-$ZnI_2$ | 3.97 | 3.23 | 2.53 (1.74) | -16.63 | $CaOH_2$-$ZnBr_2$ | 3.66 | 2.01 | 3.65 (1.64) | -8.44 |
| SiH-$ZnI_2$ | 3.94 | 2.25 | 2.45 (1.39 ) | -6.88 | $ZnCl_2$-$CaOH_2$ | 3.55 | 1.98 | 3.62 (1.76) | -9.12 |
| GaSe-SiH | 3.79 | 2.17 | 2.61 (1.24) | -8.60 | | | | | |

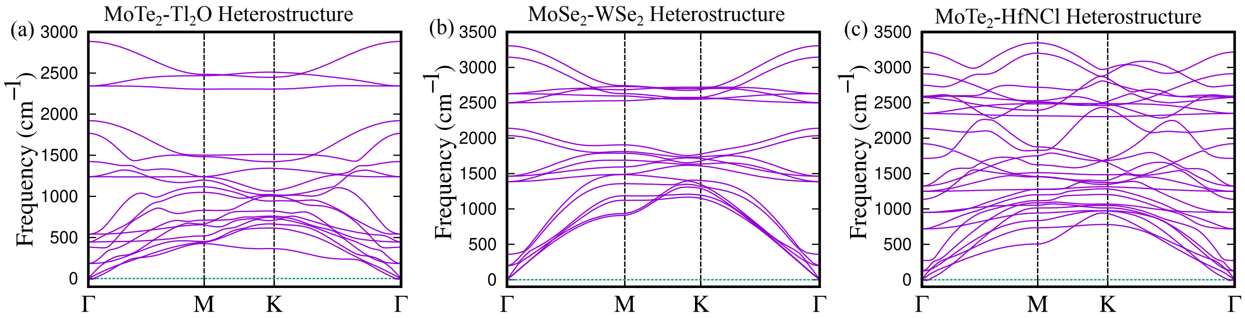


FIG. S4. Phonon dispersion of (a) $MoTe_2/Tl_2O$, (b)$MoSe_2/WSe_2$ and (c) $MoTe_2$/HfNCl heterostructures. Absence of imaginary frequencies confirms their dynamical stability.

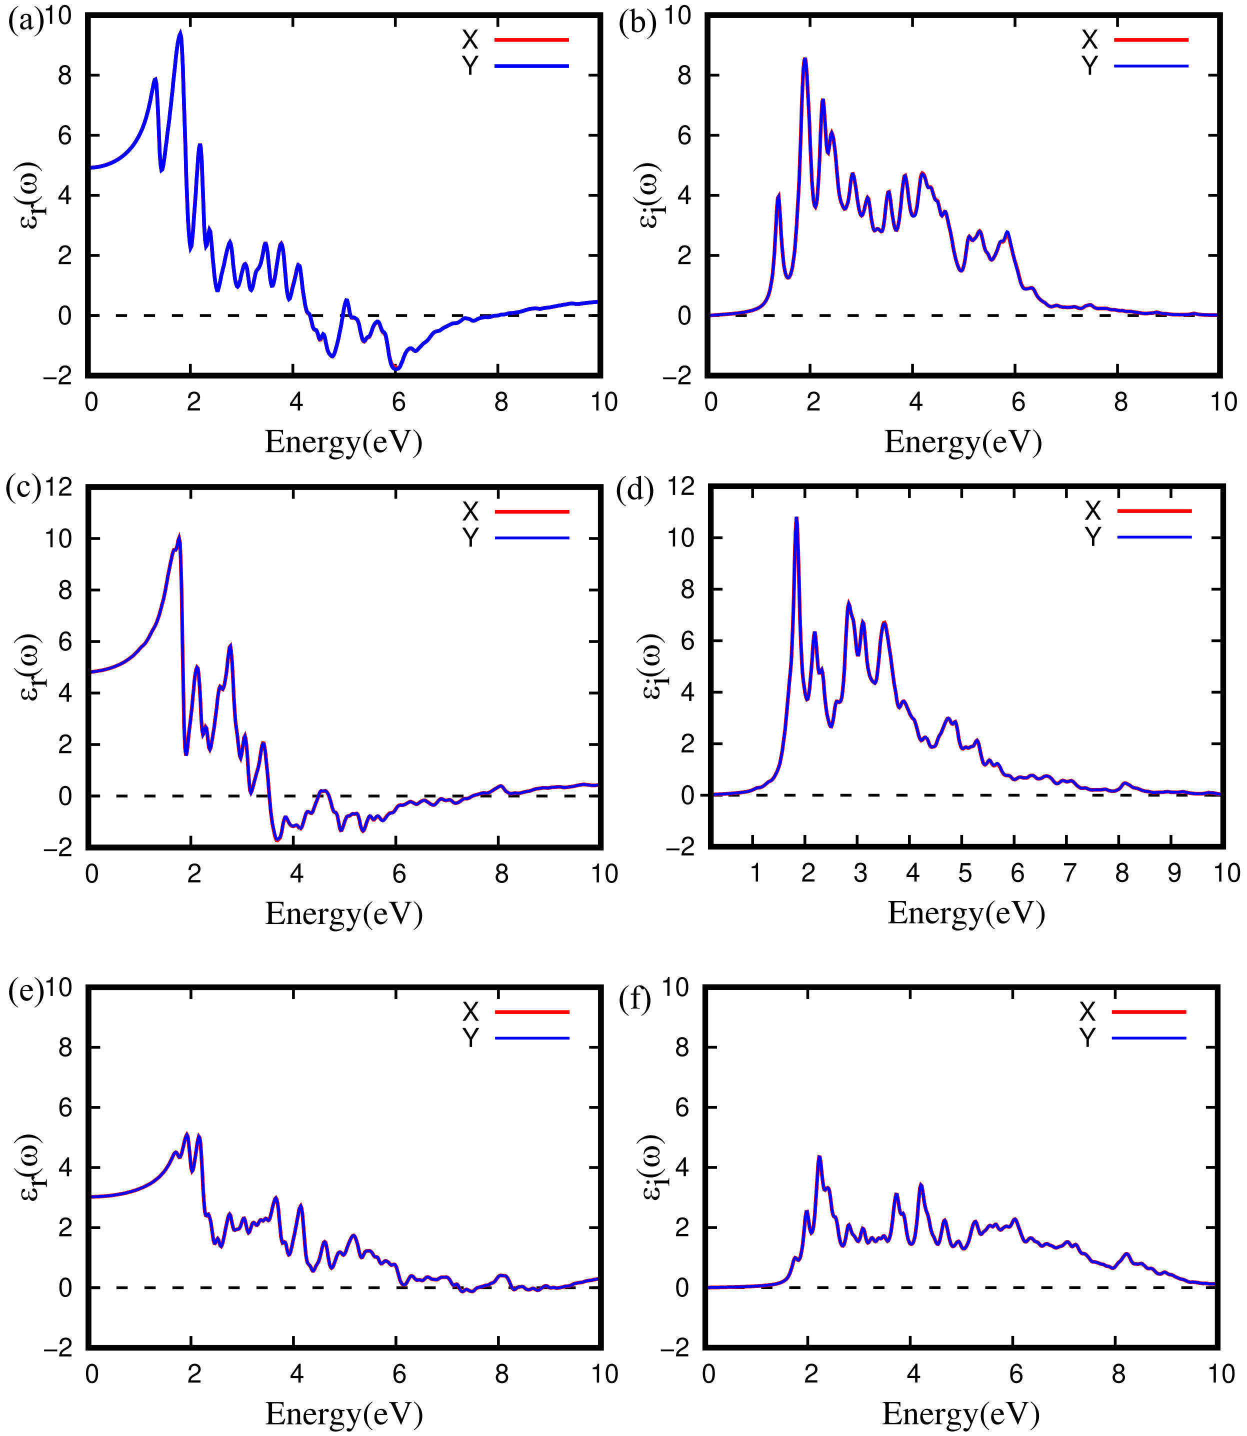


FIG. S5. (a) Real and (b) Imaginary part of the dielectric function of $MoTe_2/Tl_2O$. (c) Real and (d) Imaginary part of the dielectric function of $MoSe_2/WSe_2$. (e) Real and (f) Imaginary part of the dielectric function of $MoTe_2/HfNCl_2$.

## S2. ELECTRONIC & OPTICAL PROPERTIES OF TOP 10 HETEROSTRUCTURES

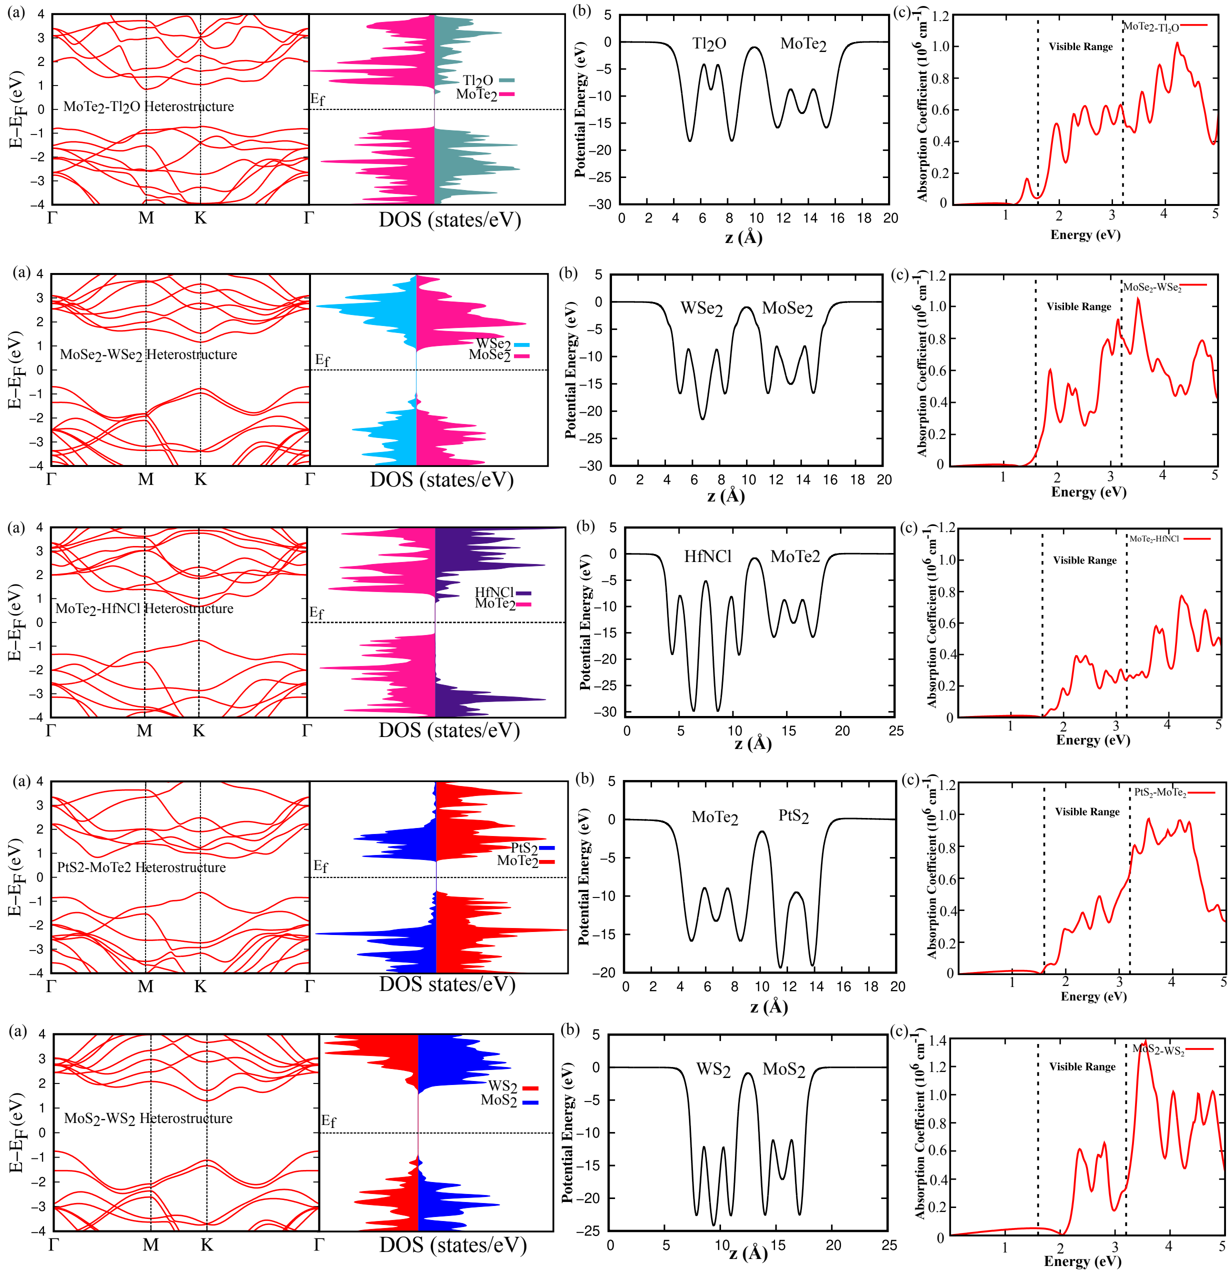


FIG. S6. Band structure, DOS, electrostatic potential energy, and absorption coefficient.

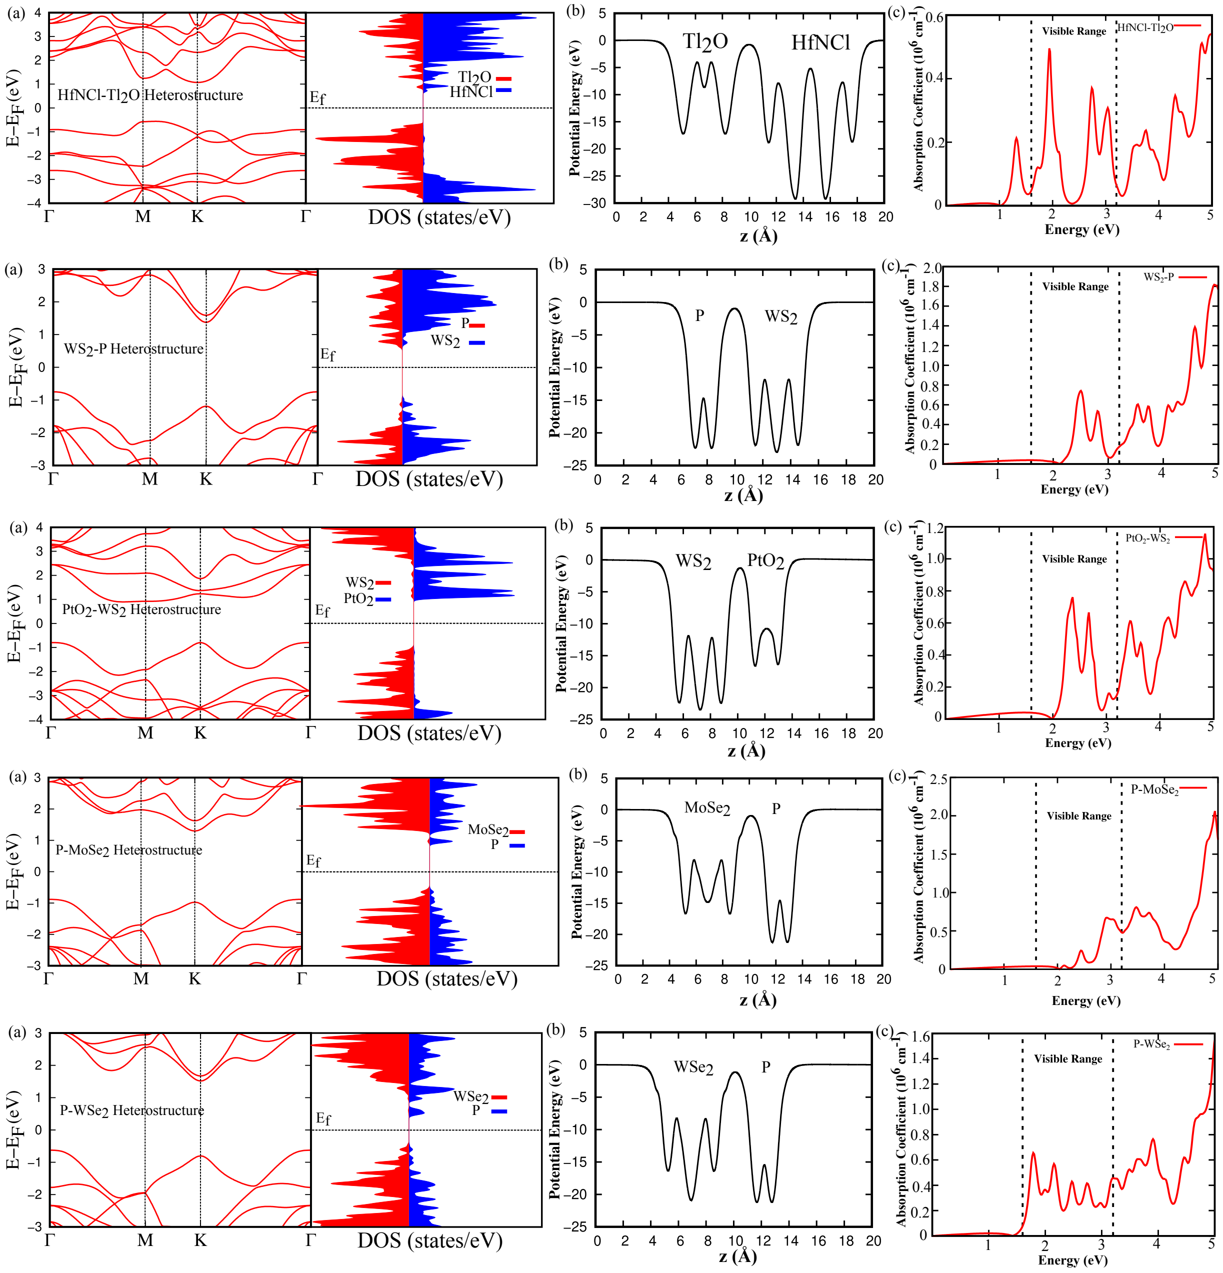


FIG. S7. Band structure, DOS, electrostatic potential energy, and absorption coefficient.

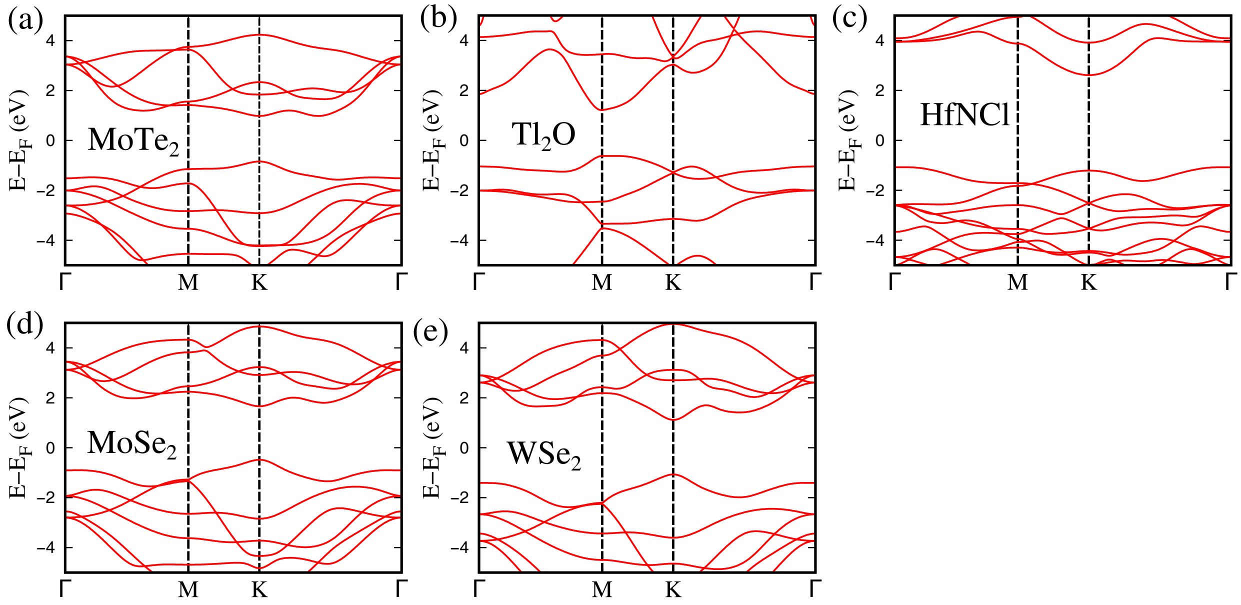


FIG. S8. Electronic band structures of monolayers: (a) $MoTe_2$, (b) $Tl_2O$, (c) HfNCl, (d) $MoSe_2$, and (e) $WSe_2$, calculated using the HSE06 hybrid functional along their respective high-symmetry paths in the Brillouin zone. Monolayers of $MoTe_2$, $MoSe_2$, and $WSe_2$ have direct band gaps. The valence band maximum (VBM) and conduction band minimum (CBM) occur at the K point in these materials. Monolayer $Tl_2O$ also exhibits a direct band gap, but its VBM and CBM are both located at the M point. In contrast, monolayer HfNCl has an indirect band gap, with the VBM at the $\Gamma$ point and the CBM at the K point. Using the GGA-PBE (HSE06) functionals, the calculated band gaps for $MoTe_2$, $Tl_2O$, HfNCl, $MoSe_2$, and $WSe_2$ are 1.10 eV (1.83 eV), 0.96 eV (1.84 eV), 2.45 eV (3.68 eV), 1.38 eV (2.13 eV), and 1.42 eV (2.19 eV), respectively. These results agree well with the previously reported values.

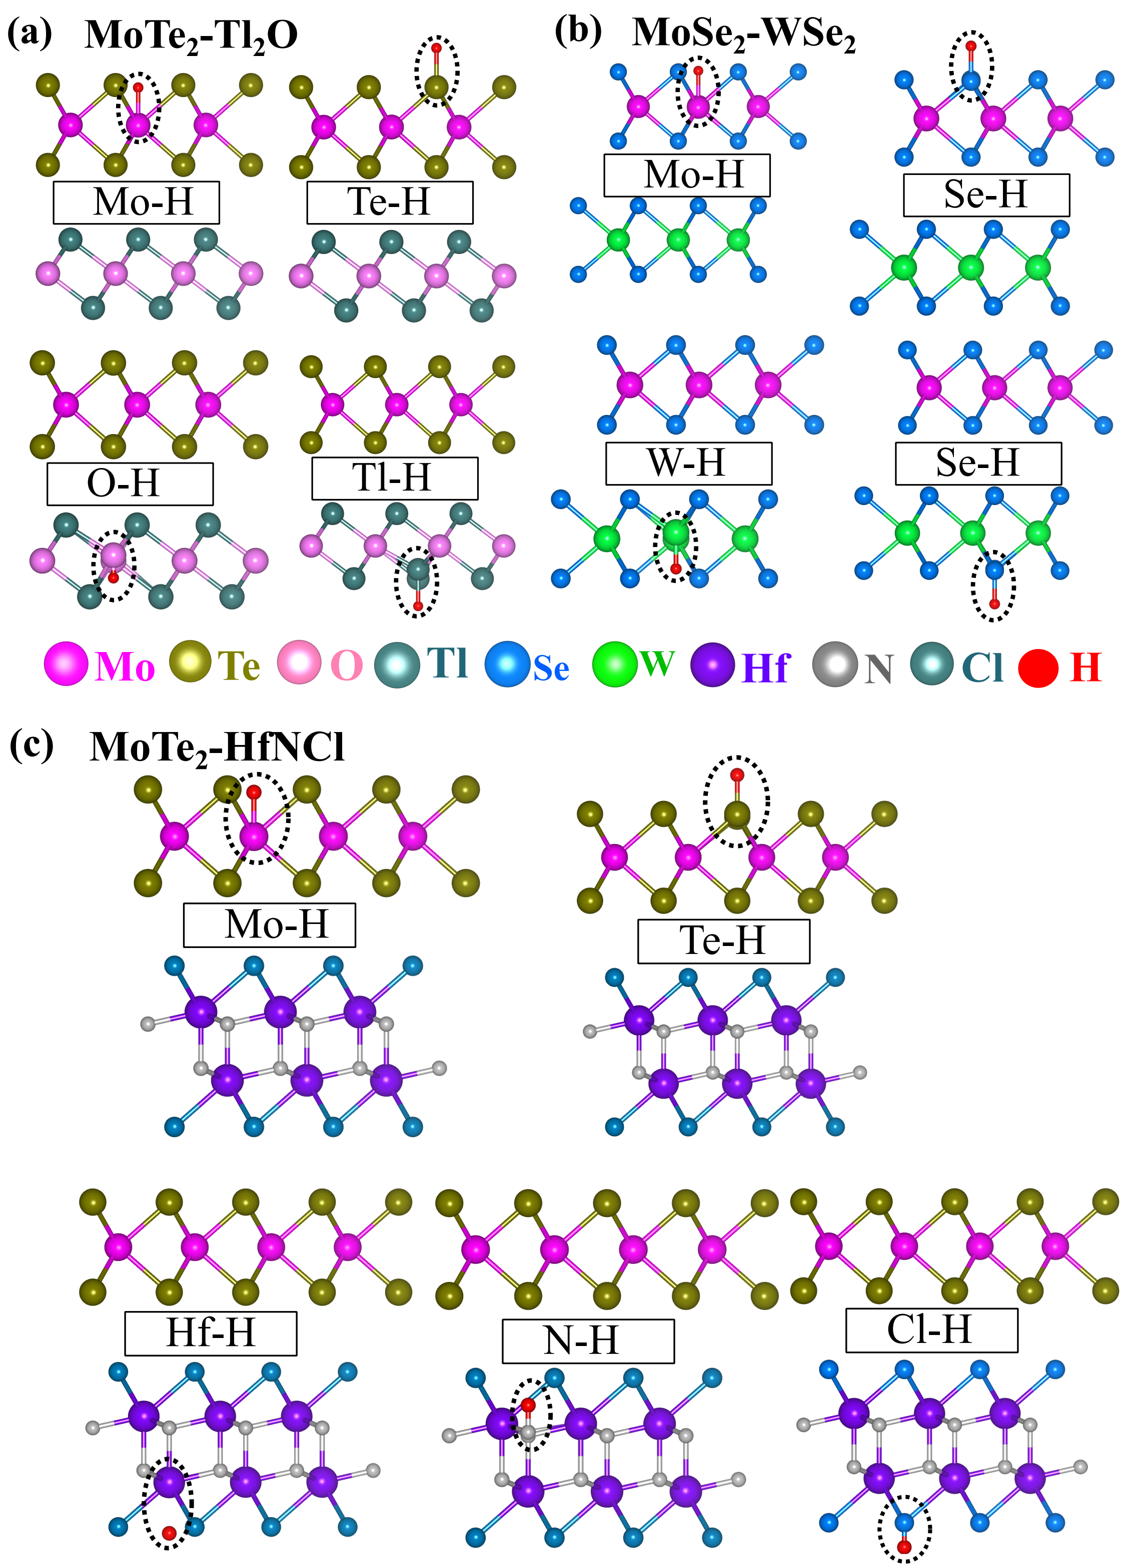


FIG. S9. The $H^*$ adsorption sites in the (a) $MoTe_2$-$Tl_2O$ heterostructure: Mo-H, Te-H, O-H, and Tl-H (b) $MoSe_2$-$WSe_2$ heterostructure: Mo-H, Se-H, W-H, and Se-H (c) $MoTe_2$-HfNCl heterostructure: Mo-H, Te-H, Hf-H, N-H, and Cl-H.
